# Supplementary material for: Learning Optimal Antenna Tilt Control Policies: A Contextual Linear Bandit Approach
Source: arXiv:2201.02169 source file (2022-01-06)
Supplement: Supplementary file 1 [file AdditionalExperiments.tex]

\newpage 
\section{Additional experimental results}
\label{app:experiments}
